# Supplementary material for: Investigation of triangularity effects on tokamak edge turbulence through multi-fidelity gyrokinetic simulations
Source: arXiv:2407.12942 source file (2024-07-17)
Supplement: Supplementary file 1 [file 991_appendix_GM_GF_equivalency.tex]

We compute the equivalency between GMs and gyrofluid moments up to the energy-weighted pressure tensor using a basis transformation from the Hermite to canonical parallel velocity space basis, $(1,\spara,\spara^2,\spara^3,\spara^4)$,
\begin{equation}
  H = \sqrt[4]{\pi} \left(
\begin{array}{ccccc}
 1 & 0 & \frac{1}{2} & 0 & \frac{3}{4} \\
 0 & \frac{1}{\sqrt{2}} & 0 & \frac{3}{2 \sqrt{2}} & 0 \\
 0 & 0 & \frac{1}{\sqrt{2}} & 0 & \frac{3}{\sqrt{2}} \\
 0 & 0 & 0 & \frac{\sqrt{3}}{2} & 0 \\
 0 & 0 & 0 & 0 & \sqrt{\frac{3}{2}} \\
\end{array}
\right),
\end{equation}
and from the Laguerre to canonical perpendicular velocity space basis, $(1,x_a,x_a^2)$,
\begin{equation}
  L = 
\left(
\begin{array}{ccc}
 1 & 1 & 2 \\
 0 & -1 & -4 \\
 0 & 0 & 2 \\
\end{array}
\right).
\end{equation}
We define the two-dimensional velocity basis transformation tensor as
\begin{equation}
    \mathsf{T_{HL}} = H^{-1}\otimes L^{-1}
\end{equation}
Any kind of product of the two canonical basis can be now written as
\begin{equation}
    \spara^m x_a^n = \bm e_m^T 
\end{equation}
